# Supplementary material for: Preliminary Study on Incremental Learning for Large Language Model-based Recommender Systems
Source: arXiv:2312.15599 source file (2024-07-30)
Supplement: Supplementary file 1 [file 8_Appendix_backup.tex]

\section{Appendix}

\subsection{Total Variation Distance}
\label{sec:appendix-tv}
%%%%%%%%%%%% todo rewrite
 We first present an introduction to the Total Variation (TV) distance, including its definition and some basic properties. 
 %before delving into the proofs of theorem~\ref{theo:tv-distance}.
% \setcounter{definition}{0}
% \begin{definition}
%     00000000
% \end{definition}
\begin{definition}[Total Variation Distance]
\label{def:TVdistance}
The total variation distance between probability measures $P$ and $Q$ on a measurable space $(\Omega, \mathcal{F})$ is defined as the supremum of the absolute difference between the probabilities assigned to a measurable event $A\in\mathcal{F}$ by $P$ and $Q$.
% \begin{equation}\small
% \label{eq:def-tv-original}
%     TV(P,Q)=\sup\limits_{A\in \mathcal{F}} \left| P(A)-Q(A)\right|.
% \end{equation}
If $\Omega$ is countable, the total variation distance can also be expressed in terms of the L1-norm~\cite{TV-distance} as follows:
\begin{equation}\small
\label{eq:tv-distance-probability}
    TV(P,Q)=\sup\limits_{A\in \mathcal{F}} \left| P(A)-Q(A)\right|=\frac{1}{2}\left \|P-Q  \right \|_{1}.
    % =\frac{1}{2}\sum_{\omega\in \Omega} \left |P(\left\{\omega \right\}) - Q(\left\{\omega \right\})  \right|.
\end{equation}
\end{definition}

% \begin{definition}
%     111111111
% \end{definition}
% \begin{definition}
%     22222222
% \end{definition}
% A computation example for TV distance can be found in Appendix~\ref{sec:appendix-proof}.


\subsection{Proofs for Theorem~\ref{theo:tv-distance}}
\label{sec:appendix-proof}
% In this subsection, we prove Theorem~\ref{theo:tv-distance} using the total variation distance and related concepts.
\setcounter{theorem}{0}
\begin{theorem}
\label{theo:tv-distance}
Given a measurable event $A$, assuming $P(S=s)=P(\hat{S}=s)$ for a given $s \in \left\{ 0,1 \right \}$, the total variation distance between two conditional probabilities $P(A|S=s)$ and $P(A|\hat{S}=s)$ is bounded by the probability that the sensitive attribute is incorrectly reconstructed, i.e., $TV(P(A|S=s), P(A|\hat{S}=s))\leq P(S\ne \hat{S}|S=s)$.
% Suppose $P(S=s)=P(\hat{S}=s)$ for a given $s \in \left\{ 0,1 \right \}$. Then $TV(p^{(s)},\hat{p}^{(s)})\leq P(S\ne \hat{S}|S=s)$
\end{theorem}


% \begin{proof}
% Given a measurable event $A$ and two conditional probabilities $P(A|S=s)$ and $P(A|\hat{S}=s)$. For simplicity and with a slight abuse of notation, we use $p_{(A|s,\hat{s})}$ to represent $P(A|S=s,\hat{S}=s)$, $p_{(A|\neg s,\hat{s})}$ to represent $P(A|S= s,\hat{S}\ne s)$, $p_{(A| s,\neg \hat{s})}$ to represent $P(A|S\ne s,\hat{S}=s)$, $p_{(A|\neg s,\hat{s})}$ to represent $P(A|S\ne s,\hat{S}=s)$ 
% Then we have:
% \notag
% \begin{small}
% \begin{alignat}{2}
%  % & \ &&\left |p^{(s)}-\hat{p}^{(s)}\right | =
%  & \quad TV(P(A|S=s),P(A|\hat{S}=s)) =  \sup_{A}\left|P(A|S=s )-P(A|\hat{S}=s) \right| \\
%  &=\sup_{A}\left| p_{(A|s,\hat{s})} p_{(\hat{s}|s)} + p_{(A|s,\neg \hat{s})} p_{(\neg\hat{s}|s)}-p_{(A|s,\hat{s})} p_{(s|\hat{s})}-p_{(A|\neg s,\hat{s})} p_{(\neg s|\hat{s})} \right| \\[-10pt]
% &=\sup_{A}\left| p_{(A|s,\hat{s})}\big(p_{(\hat{s}|s)}-p_{(s|\hat{s})} \big) - p_{(\neg\hat{s}|s)} \big(p_{(A|s,\neg \hat{s})}-p_{(A|\neg s,\hat{s})}  \big)
% \right| \\
% &=\sup_{A}\left| 0 - p_{(\neg\hat{s}|s)} \big(
% p_{(A|s,\neg \hat{s})} - p_{(A|\neg s,\hat{s})}\big)
% \right| \\
% &\leq p_{(\neg \hat{s}|s)}=P(\hat{S}\ne s|S=s)=P(\hat{S}\ne S|S=s)
% \end{alignat}
% \end{small}
% \end{proof}

\begin{proof}
Given a measurable event $A$ and two conditional probabilities $P(A|S=s)$ and $P(A|\hat{S}=s)$. We have:
\notag
\begin{small}
\begin{alignat}{2}
 % & \ &&\left |p^{(s)}-\hat{p}^{(s)}\right | =
 & \quad TV(P(A|S=s),P(A|\hat{S}=s)) =  \sup_{A}\left|P(A|S=s )-P(A|\hat{S}=s) \right| \\
 &=\sup_{A}\left| P( A|S=s,\hat{S}=s ) P( \hat{S}=s|S=s ) \text{+} P( A|S=s,\hat{S}\ne s ) P( \hat{S}\ne s|S=s ) \right.\\[-10pt]
 &\ - \left. P( A|S=s,\hat{S}= s ) P( S=s|\hat{S}=s ) - P( A|S\ne s,\hat{S}=s ) P( S\ne s|\hat{S} = s )\right| \\[-10pt]
&=\sup_{A}\left|P(A|S=s,\hat{S}=s)\left( P(\hat{S}=s|S=s) - P(S=s|\hat{S}=s)\right) \right.\\[-5pt]
&\ -\left.P(\hat{S}\ne S|S=s)\left(P(A|S=s,\hat{S}\ne s)-P(A|\hat{S}=s,S\ne s) \right)\right|\\[-2pt]
&=\sup_{A}\left| 0 - P(\hat{S}\ne S|S=s) \left(P(A|S=s,\hat{S}\ne s) - P(A|\hat{S}=s.S\ne s) \right)\right| \\[-8pt]
&\leq P(\hat{S}\ne S|S=s).
\end{alignat}\end{small}
\vspace{-5pt}
\end{proof}


% \begin{proof}
% Given a measurable event $A$ and two conditional probabilities $P(A|S=s )$ and $P(A|\hat{S}=s)$, we have:
% \notag
% \begin{alignat}{2}\small
%  % & \ &&\left |p^{(s)}-\hat{p}^{(s)}\right | =
%  & \quad TV(P(A|S=s),P(A|\hat{S}=s)) =  \sup_{A}\left|P(A|S=s )-P(A|\hat{S}=s) \right| \\
%  &=\sup_{A}\left| P( A|S=s,\hat{S}=s ) P( \hat{S}=s|S=s ) \text{+} P( A|S=s,\hat{S}\ne s ) P( \hat{S}\ne s|S=s ) \right.\\
%  &\ - \left. P( A|S=s,\hat{S}= s ) P( S=s|\hat{S}=s ) - P( A|S\ne s,\hat{S}=s ) P( S\ne s|\hat{S} = s )\right| \\
% &=\sup_{A}\left|P(A|S=s,\hat{S}=s)\left( P(\hat{S}=s|S=s) - P(S=s|\hat{S}=s)\right) \right.\\
% &\ -\left.P(\hat{S}\ne S|S=s)\left(P(A|S=s,\hat{S}\ne s)-P(A|\hat{S}=s,S\ne s) \right)\right|\\
% &=\sup_{A}\left| 0 - P(\hat{S}\ne S|S=s) \left(P(A|S=s,\hat{S}\ne s) - P(A|\hat{S}=s.S\ne s) \right)\right| \\
% &\leq P(\hat{S}\ne S|S=s)
% \end{alignat}
% % \begin{alignat}{2}
% %     \left| p^{(s)}-\hat{p}^{(s)}\right | &= \left|P(A|S=s)-P(A|\hat{S}=s) \right|\ \\
% %        &= &&\left|P(A|S=s)\\
% %        &&-P(A|\hat{S}=s)\right|
% % \end{alignat}
% \end{proof}
